# Supplementary material for: Multi-channel exchange-scattering spin polarimetry
Source: arXiv:1506.04239 source file (2015-06-13)
Supplement: Supplementary file 1 [file MCVLEED_SM.pdf]

# Multi-channel exchange-scattering spin polarimetry

Fuhao Ji[2], Tan Shi[2], Mao Ye[1], Weishi Wan[3], Zhen Liu[2], Jiajia Wang[4], Tao Xu[4], and Shan Qiao[1,4,*]

[1]*State Key Laboratory of Functional Materials for Informatics, Shanghai Institute of Microsystem and Information Technology, Chinese Academy of Sciences, 865 Changning Road, Shanghai 200050, China*

[2] *Physics Department, Laboratory of advanced Materials, and Surface Physics Laboratory (National Key Laboratory), Fudan University, 2005 songhu road, Shanghai, 200438, China*

[3] *Advanced Light Source, Lawrence Berkeley National Laboratory, 1 Cyclotron Road, Berkeley, CA 94720, USA*

[4] *School of physical science and technology, ShanghaiTech University, 319 Yueyang Road, Shanghai, 200031, China*

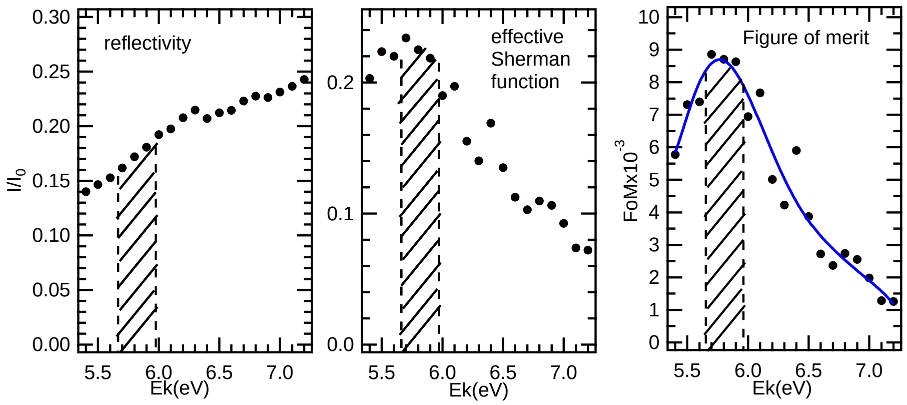


FIG. 1. The average reflectivity, effective Sherman function and figure of merit of the spin polarimeter under different central reflecting energies. Shadowed area represents the practical energy window adopted.

When passing through magnetic field, the projection of electron spin along magnetic field direction is conserved and that perpendicular to that undergoes a Larmor precession with a frequency

$$\omega_s = eB/m$$

On the other hand, the electron orbital frequency $\omega_0$ can be estimated to be the ratio between its velocity and orbital radius R

$$\omega_0 = v/R = ((eBR/m))/R = eB/m$$

Which is the same as $\omega_s$. So the projection of electron spin perpendicular to the magnetic field will turn just 180 degree and the Larmor procession does not destroy the function of the spin polarimeter.

To achieve the best performance, the dependence of $S_{eff}$ and $I/I_0$ on scattering energy need to be studied. Figure 1 shows the measured average reflectivity $I/I_0$, effective Sherman function $S_{eff}$ and the corresponding Figure of Merit $FOM = (I/I_0) * S_{eff}^2$ with different central scattering energies. The typical energy window adopted in a multichannel spin detection is 375meV, which leads a significant changing of both reflectivity and effective Sherman function across the energy window. The optimal center scattering energy is found to be 5.8 eV, which gives an average $< FOM >$ of $8.5 \times 10^{-3}$.

* qiaoshan@mail.sim.ac.cn;
